# Supplementary material for: System and Method to Determine ME/CFS and Long COVID Disease Severity Using a Wearable Sensor
Source: arXiv:2404.04345 source file (2024-04-05)
Supplement: Supplementary file 1 [file supplementary-materials.tex]

\section*{Supplementary Materials}

\textcolor{red}{*** I think this paragraph should go in Supplementary Materials ***  Additional Parameters using tsfresh: tsfresh is a powerful Python library designed for automatic time series feature extraction \cite{tsfresh} based on the FeatuRe Extraction and Scalable Hypothesis testing (FRESH) \cite{fresh} algorithm. It combines algorithms from various domains, such as statistics, time-series analysis, signal processing, and nonlinear dynamics, with a robust feature selection algorithm. By integrating tsfresh into MetaProcessor, we provide users with three options for feature extraction: minimal feature settings, efficient feature settings, and comprehensive feature settings \footnote{The feature extraction settings are provided by \texttt{tsfresh}: \url{https://tsfresh.readthedocs.io/en/latest/api/tsfresh.feature\_extraction.html\#module-tsfresh.feature\_extraction.settings}.}. This automated feature engineering process saves time and effort, allowing researchers to focus on other tasks. However, it is important to note that tsfresh is limited to CPU-based computation, which can result in lengthy processing times for large datasets. Users should be aware of this limitation and plan their feature extraction tasks accordingly (results derived from the use of tsfresh are included in the Supplementery Materials).}

The Figures \ref{fig:ai}, \ref{fig:rhi}, and \ref{fig:hr} were produced using standardized survey data collected from study participants during their visits to The Bateman Horne Center, as well as data collected through online forms. While we did not formulate specific hypotheses for each of the features depicted in these figures, we have the necessary tools and data to generate them. As such, we have included these figures for future reference.
Included features are: Augmentation Index (AI), Augmentation Index Normalized to HR 75 bpm (AI75), Baseline Heart Rate (bpm) (BLHR), Natural Base Log of Reactive Hyperemia Index (LnRHI), Reactive Hyperemia Index (RHI), and Hours of Upright Activity (HUA).

\begin{figure*}
\centering
\includegraphics[width=7.16in]{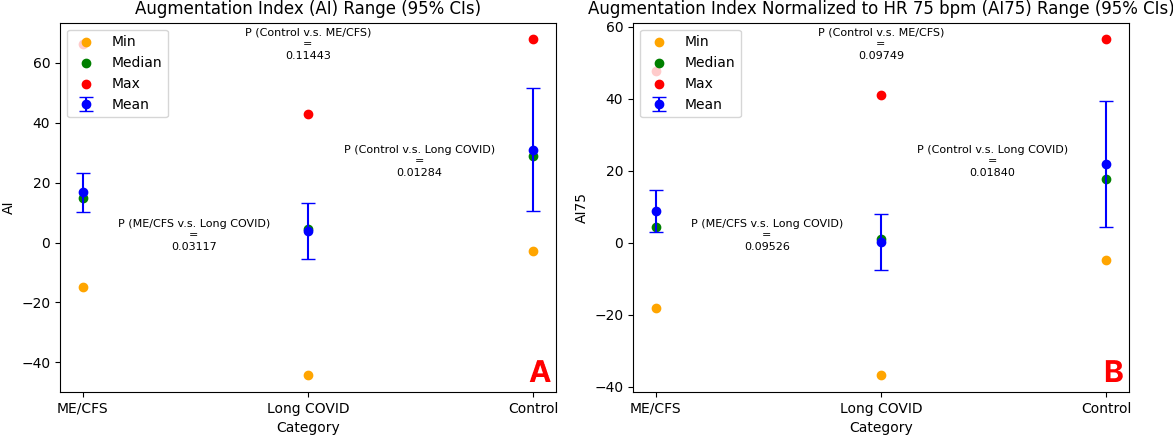}
\caption{Grouped t-test performed at 95\% confidence level for Augmentation Index, and Augmentation Index Normalized to HR 75 bpm. ME/CFS vs. Long COVID vs. Control. In the legend, “Mean” is mean plus or minus a standard error.}
\label{fig:ai}
\end{figure*}

\begin{figure*}
\centering
\includegraphics[width=7.16in]{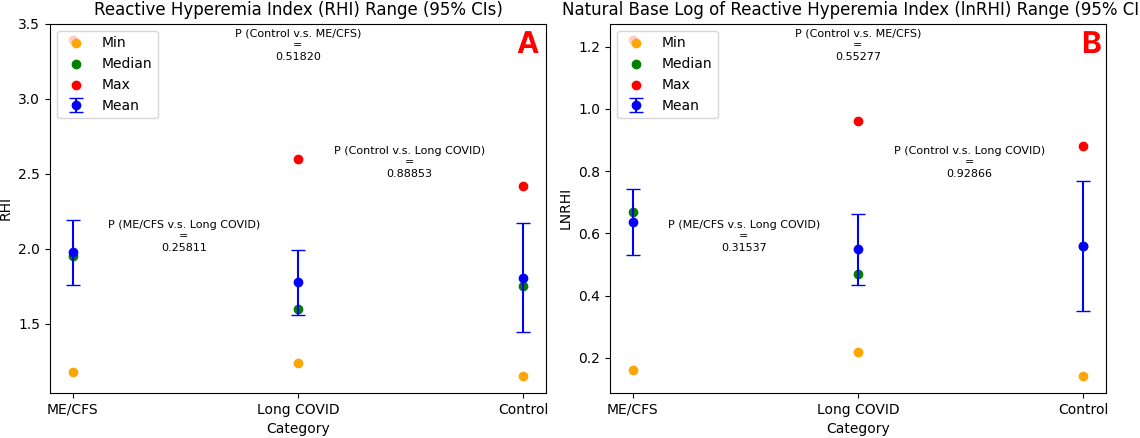}
\caption{Grouped t-test performed at 95\% confidence level for Reactive Hyperemia Index, and Natural Base Log of Reactive Hyperemia Index. ME/CFS vs. Long COVID vs. Control. In the legend, “Mean” is mean plus or minus a standard error.}
\label{fig:rhi}
\end{figure*}

\begin{figure}
\centering
\includegraphics[width=3.5in]{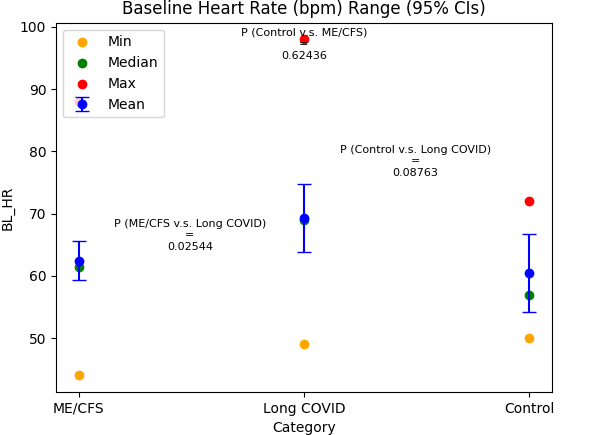}
\caption{Grouped t-test performed at 95\% confidence level for Baseline Heart Rate (bpm). ME/CFS vs. Long COVID vs. Control. In the legend, “Mean” is mean plus or minus a standard error.}
\label{fig:hr}
\end{figure}

We extracted a large number of features from the time series data using \texttt{tsfresh}, but we didn't utilize it to its full extent. \texttt{tsfresh} is benchmarked and showed good results with small datasets, meaning the row number of the testing datasets are relatively small (mostly less than 10 thousand rows), which may not be applicable to our EndoPAT study data as each of our data point averaged around 15 million rows, containing complex patterns and noises. Additionally, the feature extraction process with \texttt{tsfresh} requires a considerable amount of computational resources when running on larger datasets, which may not be feasible for our purpose. In our test runs, with the ``basic feature" \footnote{Defined as \texttt{MinimalFCParameters} in \texttt{tsfresh}.} settings (60 columns, 10 columns each for 3-axis accelerometer data and 3-axis gyroscope data), the calculation lasted around 1 minute per patient day, and for the  ``efficient feature" \footnote{Defined as \texttt{EfficientFCParameters} in \texttt{tsfresh}.} settings (about 4700 columns) calculation lasted from 49 hours per patient day to 169 hours per patient day \footnote{The unit, ``patient day" is defined as 24 hours worth of the study participants' accelerometer and gyroscope data, for example, if we collected 7 days of sensor data for 2 study participant, we'll have 14 ``patient days" worth of data.}.

\begin{table}[!ht]
\begin{center}
\begin{tabular}{|l|l|l|l|l|l|l|l|}
\hline
\textbf{Feature}             & \textbf{$A_x$}  & \textbf{$A_y$} & \textbf{$A_z$}  & \textbf{$G_x$}  & \textbf{$G_y$}  & \textbf{$G_z$}  \\ \hline
\texttt{sum\_values}         & \color{cyan}{R} & N              & \color{cyan}{R} & N               & \color{cyan}{R} & N               \\ \hline
\texttt{median}              & \color{cyan}{R} & N              & \color{cyan}{R} & N               & \color{cyan}{R} & N               \\ \hline
\texttt{mean}                & \color{cyan}{R} & N              & \color{cyan}{R} & N               & \color{cyan}{R} & N               \\ \hline
\texttt{length}              & N               & N              & N               & N               &   N             & N               \\ \hline
\texttt{standard\_deviation} & \color{cyan}{R} & N              & \color{cyan}{R} & N               & \color{cyan}{R} & N               \\ \hline
\texttt{variance}            & \color{cyan}{R} & N              & \color{cyan}{R} & N               & \color{cyan}{R} & N               \\ \hline
\texttt{root\_mean\_square}  & \color{green}{S}& N              & \color{green}{S}& \color{cyan}{R} & \color{green}{S}&\color{cyan}{R} \\ \hline
\texttt{maximum}             & N               & N              & N               & N               &   N             & N               \\ \hline
\texttt{absolute\_maximum}   & N               & N              & N               & N               &   N             & N               \\ \hline
\texttt{minimum}             & N               & N              & N               & N               &   N             & N               \\ \hline
\end{tabular}
\end{center}
% ax, az, for sum, medium and rms should be significant disease severity while ay should not be, gy should be a significant predictor of movement activity (especially rms), variance for acce and gyro should be predictive of activity level
\caption{Analysis on tsfresh MinimalFCParameters. $A_{x|y|z}$ and $G_{x|y|z}$ corresponds to accelerometer's and gyroscope's axis. ``S" (in green) - might have strong correlation; ``R" (in blue) - might have correlation; ``N" (in black) - should not have any correlation.}
\label{table:tsfresh}
\end{table}

Using the ``basic features" calculated with \texttt{tsfresh}, we classified the 60 output features into different groups: possible strong correlation, possible correlation, and theoretically not possible to have any correlation (Table \ref{table:tsfresh}. Our reasoning behind is due to the wearing orientation of MMS devices: forward corresponds to x-axis of IMU, vertical corresponds to y-axis of IMU, and left corresponds to z-axis of IMU. 

The forward x-axis and left z-axis directions of the IMU, represented by $A_x$ and $A_z$, are expected to demonstrate some correlation with disease severity when considering sum, medium, and RMS values. This is because these axes capture the horizontal and lateral movements during daily activities, which are likely to be affected in patients experiencing orthostatic intolerance, fatigue, and other symptoms common in ME/CFS and Long COVID.

On the other hand, the vertical direction, y-axis, represented by $A_y$, should not have a significant correlation with disease severity. This is because the y-axis mainly captures gravitational forces and is less informative in capturing the specific movements and postural changes that are relevant to these conditions.

$G_y$ represents the angular velocity of the gyroscopic sensor, is expected to be a significant predictor of movement activity, particularly when considering RMS values. This is because the RMS values effectively capture the variations in movement intensity, which can be informative in assessing the overall activity levels of the patients.

Lastly, the variance for both acceleration and angular velocity should be predictive of activity levels. Higher variances in these measurements indicate a broader range of motion and more diverse movement patterns, which can be associated with higher activity levels in patients. Conversely, lower variances suggest reduced motion and a more limited range of activities, which can be indicative of lower activity levels commonly observed in patients with ME/CFS and Long COVID.

\begin{table*}
\begin{center}
\begin{tabular}{|l|l|l|l|l|l|l|l|}
\hline
\textbf{Feature}             & \textbf{$A_x$}          & \textbf{$A_y$} & \textbf{$A_z$}          & \textbf{$G_x$}         & \textbf{$G_y$}     & \textbf{$G_z$}    \\ \hline
\texttt{sum\_values}         & \color{cyan}{0.041924}  &      0.0       & \color{cyan}{0.191563}  & 0.000187               & \color{cyan}{0.000523} &      0.0      \\ \hline
\texttt{median}              & \color{cyan}{0.015792}  &      0.0       & \color{cyan}{0.228202}  & 0.647568               & \color{cyan}{0.006879} & 0.000005      \\ \hline
\texttt{mean}                & \color{cyan}{0.041332}  &      0.0       & \color{cyan}{0.187355}  &  0.00018               & \color{cyan}{0.000533} &      0.0      \\ \hline
\texttt{length}              & 0.000035                & 0.000035       & 0.000035                & 0.000035               & 0.000035           & 0.000035          \\ \hline
\texttt{standard\_deviation} & \color{cyan}{0.159109}  & 0.000353       & \color{cyan}{0.005491}  & 0.027135               & \color{cyan}{0.0}  &      0.0          \\ \hline
\texttt{variance}            & \color{cyan}{0.110206}  & 0.000389       & \color{cyan}{0.004282}  & 0.011215               & \color{cyan}{0.0}  &      0.0          \\ \hline
\texttt{root\_mean\_square}  & \color{green}{0.000826} &      0.0       & \color{green}{0.000138} & \color{cyan}{0.027227} & \color{green}{0.0} & \color{cyan}{0.0} \\ \hline
\texttt{maximum}             & 0.836597                & 0.013301       & 0.690229                & 0.114135               &  0.07336           & 0.198528          \\ \hline
\texttt{absolute\_maximum}   & 0.020304                & 0.021652       & 0.412479                & 0.073017               & 0.202262           & 0.043988          \\ \hline
\texttt{minimum}             & 0.002246                & 0.829734       & 0.412457                & 0.020094               & 0.333653           & 0.031144          \\ \hline
\end{tabular}
\end{center}
\caption{T-Tests for features gendered on tsfresh MinimalFCParameters: Control vs. ME/CFS $p$-value table. ``S" (in green) - might have strong correlation; ``R" (in blue) - might have correlation; ``N" (in black) - should not have any correlation.}
\label{table:tsfresh-control-vs-mecfs}
\end{table*}

\begin{table*}
\begin{center}
\begin{tabular}{|l|l|l|l|l|l|l|l|}
\hline
\textbf{Feature}             & \textbf{$A_x$}         & \textbf{$A_y$} & \textbf{$A_z$}          & \textbf{$G_x$}         & \textbf{$G_y$}          & \textbf{$G_z$}         \\ \hline
\texttt{sum\_values}         & \color{cyan}{0.472635} & 0.00005        & \color{cyan}{0.269436}  & 0.099531               & \color{cyan}{0.425181}  & 0.000004               \\ \hline 
\texttt{median}              & \color{cyan}{0.641273} & 0.000002       & \color{cyan}{0.196691}  & 0.957038               & \color{cyan}{0.541774}  & 0.001393               \\ \hline 
\texttt{mean}                & \color{cyan}{0.46812}  & 0.000073       & \color{cyan}{0.269345}  & 0.10009                & \color{cyan}{0.428071}  & 0.000005               \\ \hline 
\texttt{length}              & 0.000034               & 0.000034       & 0.000034                & 0.000034               & 0.000034                & 0.000034               \\ \hline 
\texttt{standard\_deviation} & \color{cyan}{0.012679} & 0.097511       & \color{cyan}{0.000537}  & 0.024193               & \color{cyan}{0.002971}  & 0.003611               \\ \hline 
\texttt{variance}            & \color{cyan}{0.020627} & 0.097818       & \color{cyan}{0.000769}  & 0.011676               & \color{cyan}{0.002415}  & 0.004402               \\ \hline 
\texttt{root\_mean\_square}  & \color{green}{0.01226} & 0.000003       & \color{green}{0.000904} & \color{cyan}{0.024315} & \color{green}{0.002977} & \color{cyan}{0.003609} \\ \hline 
\texttt{maximum}             & 0.437505               & 0.028048       & 0.21497                 & 0.802929               & 0.01724                 & 0.89266                \\ \hline 
\texttt{absolute\_maximum}   & 0.097325               & 0.037574       & 0.131244                & 0.828048               & 0.053146                & 0.697704               \\ \hline 
\texttt{minimum}             & 0.066436               & 0.934615       & 0.133253                & 0.775239               & 0.340476                & 0.363448               \\ \hline 
\end{tabular}
\end{center}
\caption{T-Tests for features gendered on tsfresh MinimalFCParameters: Control vs. Long COVID $p$-value table. ``S" (in green) - might have strong correlation; ``R" (in blue) - might have correlation; ``N" (in black) - should not have any correlation.}
\label{table:tsfresh-control-vs-longcovid}
\end{table*}       

\begin{table*}
\begin{center}
\begin{tabular}{|l|l|l|l|l|l|l|l|}
\hline
\textbf{Feature}             & \textbf{$A_x$}          & \textbf{$A_y$} & \textbf{$A_z$}          & \textbf{$G_x$}         & \textbf{$G_y$}          & \textbf{$G_z$}         \\ \hline
\texttt{sum\_values}         & \color{cyan}{0.032805}  & 0.010449       & \color{cyan}{0.599469}  & 0.073061               & \color{cyan}{0.000482}  & 0.365713               \\ \hline
\texttt{median}              & \color{cyan}{0.002744}  & 0.00173        & \color{cyan}{0.685771}  & 0.642964               & \color{cyan}{0.01127}   & 0.921931               \\ \hline
\texttt{mean}                & \color{cyan}{0.03251}   & 0.009921       & \color{cyan}{0.589232}  & 0.071567               & \color{cyan}{0.000463}  & 0.361612               \\ \hline
\texttt{length}              & 0.589508                & 0.589508       & 0.589508                & 0.589508               & 0.589508                & 0.589508               \\ \hline
\texttt{standard\_deviation} & \color{cyan}{0.328658}  & 0.000856       & \color{cyan}{0.989138}  & 0.756259               & \color{cyan}{0.020668}  & 0.003687               \\ \hline
\texttt{variance}            & \color{cyan}{0.494278}  & 0.001406       & \color{cyan}{0.723901}  & 0.519591               & \color{cyan}{0.012312}  & 0.001817               \\ \hline
\texttt{root\_mean\_square}  & \color{green}{0.071836} & 0.000092       & \color{green}{0.124049} & \color{cyan}{0.756988} & \color{green}{0.020627} & \color{cyan}{0.003683} \\ \hline
\texttt{maximum}             & 0.15072                 & 0.910401       & 0.293532                & 0.011299               & 0.508641                & 0.155688               \\ \hline
\texttt{absolute\_maximum}   & 0.711243                & 0.776089       & 0.392233                & 0.004648               & 0.403723                & 0.046802               \\ \hline
\texttt{minimum}             & 0.287907                & 0.688138       & 0.310116                & 0.004312               & 0.972233                & 0.171762               \\ \hline
\end{tabular}
\end{center}
\caption{T-Tests for features gendered on tsfresh MinimalFCParameters: ME/CFS vs. Long COVID $p$-value table. ``S" (in green) - might have strong correlation; ``R" (in blue) - might have correlation; ``N" (in black) - should not have any correlation.}
\label{table:tsfresh-mecfs-longcovid}
\end{table*}   

Upon conducting grouped t-tests (Tables \ref{table:tsfresh-control-vs-mecfs}, \ref{table:tsfresh-control-vs-longcovid}, \ref{table:tsfresh-mecfs-longcovid}), we noticed promising results for most parameters marked as having possible correlation and possible strong correlation across all groups. However, further in-depth analysis is required to draw more concrete conclusions.

As \texttt{tsfresh} is not the primary focus of our research, we included all results of grouped t-tests in the tables and encourage interested readers to explore this area further for a more comprehensive understanding of the relationships between these features and the conditions under study. Future work in this area could potentially reveal additional insights into the utility of these features as potential biomarkers for disease severity and activity levels in patients with ME/CFS and Long COVID with overall lower computation cost.
